# Supplementary material for: Towards Practical Verification of Machine Learning: The Case of Computer Vision Systems
Source: arXiv:1712.01785 source file (2022-12-20)
Supplement: Supplementary file 1 [file appendix_old.tex]

\begin{appendix}
\begin{comment}
\subsection{Parameter space reduction for transformation composition}
For some transformations having small number of transformation states, their composition can also be checked efficiently, as detailed in Section~\ref{sec:eval}.
For transformations having relative large number of states, even in polynomial with input size (\eg $O(n^3)$), can be prohibitively expensive to verify in practice after being composed (\ie shear and scale \cf Table~\ref{tab:bounds}).
Therefore, how to further reduce the state space for transformation combination becomes an interesting problem.

As a first step, we show in this paper that we can reduce part of the critical states by leveraging some property of the transformation \ie matrix multiplication.
In particular, we prove in previous example (reflection then rotation) which has $3r$ total states can be reduced to checking only $r$.
Let us reconsider the affine transformations. In this case it essentially computes $T_{refl}\cdot (T_{rot}\cdot G)=(T_{refl}\cdot T_{rot})\cdot G$ where G is the grid of coordinates of input image.
We add one dummy row $[0,0,1]$ at the bottom of each transformation matrix $T$ to maintain the dimensionality of transformed input grid $G$.
Then we have the compositional transformation matrix $T_{comp}=T_{refl}\cdot T_{rot}$ equals to:
\begin{equation*}
\renewcommand{\arraystretch}{1}
\setlength\arraycolsep{3pt}
\begin{aligned}
&Horizontal:\\
  &\begin{bmatrix}
    -1 & 0 & 0 \\
    0 & 1 & 0 \\
    0 & 0 & 1 
  \end{bmatrix}
  \begin{bmatrix}
    \cos\theta & -\sin\theta & 0 \\
    \sin\theta & \cos\theta & 0 \\
    0 & 0 & 1
  \end{bmatrix}=
  \begin{bmatrix}
    -\cos\theta & \sin\theta & 0 \\
    \sin\theta & \cos\theta & 0 \\
    0 & 0 & 1
  \end{bmatrix}
\\
&Vertical:\\
  &\begin{bmatrix}
    1 & 0 & 0 \\
    0 & -1 & 0 \\
    0 & 0 & 1 
  \end{bmatrix}
  \begin{bmatrix}
    \cos\theta & -\sin\theta & 0 \\
    \sin\theta & \cos\theta & 0 \\
    0 & 0 & 1
  \end{bmatrix}=
  \begin{bmatrix}
    \cos\theta & -\sin\theta & 0 \\
    -\sin\theta & -\cos\theta & 0 \\
    0 & 0 & 1
  \end{bmatrix}
\\
&Central:\\
  &\begin{bmatrix}
    -1 & 0 & 0 \\
    0 & -1 & 0 \\
    0 & 0 & 1 
  \end{bmatrix}
  \begin{bmatrix}
    \cos\theta & -\sin\theta & 0 \\
    \sin\theta & \cos\theta & 0 \\
    0 & 0 & 1
  \end{bmatrix}=
  \begin{bmatrix}
    -\cos\theta & \sin\theta & 0 \\
    -\sin\theta & -\cos\theta & 0 \\
    0 & 0 & 1
  \end{bmatrix}
\end{aligned}
\end{equation*}
where horizontal, vertical and original corresponds to reflection directions.
Then it is easy to get that horizontal reflection with rotation degree $\theta$ is equal to vertical reflection with rotation degree $\theta+180^{\circ}$.
Likewise, reflection with respect to central then rotate $\theta$ is same as simply rotate $\theta+180^{\circ}$.
Therefore, we only need to consider either horizontal or vertical reflection, without the need to check both as all rotation degrees covered by one is exactly $\pm 180^{\circ}$ of another.
If we have checked all $\theta$ from $0^{\circ}$ to $360^{\circ}$ with horizontal reflection, then we have checked all $\theta$ from $180^{\circ}$ to $540^{\circ}$, which is the same as rotating from $0^{\circ}$ to $360^{\circ}$.
Same ideas applies to reflection with respect to central, as it is essentially a $180^{\circ}$ rotation, after rotating $\theta$ and then rotate $180^{\circ}$ covers the same rotation effects if we consider all $\theta$ from $0^{\circ}$ to $360^{\circ}$.
Assume we have already checked all possible rotation degrees $r$ (without composition), then now we only need consider another $r$ states with either horizontal or vertical reflection.
This is enough to cover all possible critical states of the composition of rotation and then reflection.
\end{comment}

\subsection{Some sample safety property violations found by \sys.}
\label{subsec:appendx}

\begin{table*}
\setlength{\tabcolsep}{12pt}
\footnotesize
\centering
\renewcommand{\arraystretch}{1.1}
\caption{Violations of transformation-invariant properties on ImageNet for different models and transformations.}
\label{tab:violations_imagenet}
\begin{tabular}{c|cc|cc|c}
\multirow{2}{*}{\textbf{Model ID}} & \multicolumn{2}{c|}{\textbf{Original}} & \multicolumn{2}{c|}{\textbf{Transformed}} & \multicolumn{1}{c}{\multirow{2}{*}{\textbf{Violated}}} \\
 & \textit{Image} & \textit{Labels (Top-5)} & \textit{Image} & \textit{Label (Top-1)} & \multicolumn{1}{c}{} \\ \hline
IMG\_C1 & \vspace{.01cm} \includegraphics[width=0.2\columnwidth,height=0.2\columnwidth,valign=c]{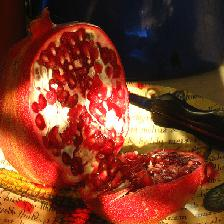}\vspace{.01cm} 
& \begin{tabular}[c]{@{}c@{}}pomegranate\\ bell\_pepper\\ acorn\_squash\\ pizza\\ trifle\end{tabular} & \vspace{.01cm} \includegraphics[width=0.2\columnwidth,height=0.2\columnwidth,valign=c]{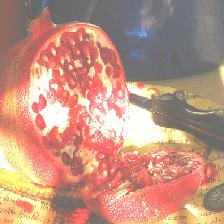}\vspace{.01cm} 
& starfish & $\phi_6$ \\ \hline
IMG\_C2 & \vspace{.01cm} \includegraphics[width=0.2\columnwidth,height=0.2\columnwidth,valign=c]{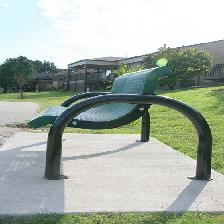}\vspace{.01cm} & \begin{tabular}[c]{@{}c@{}}park\_bench\\ sundial\\ cannon\\ bannister\\ plow\end{tabular} & \vspace{.01cm} \includegraphics[width=0.2\columnwidth,height=0.2\columnwidth,valign=c]{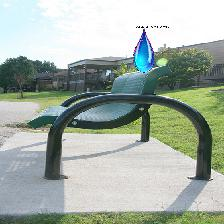}\vspace{.01cm} & peacock & $\phi_7$ \\ \hline
IMG\_C3 & \vspace{.01cm} \includegraphics[width=0.2\columnwidth,height=0.2\columnwidth,valign=c]{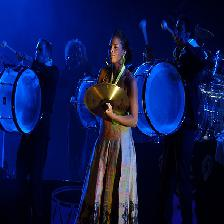}\vspace{.01cm} & \begin{tabular}[c]{@{}c@{}}stage\\ cornet\\ trombone\\ cello\\ violin\\ bathtub\end{tabular} & \vspace{.01cm} \includegraphics[width=0.2\columnwidth,,height=0.2\columnwidth,valign=c]{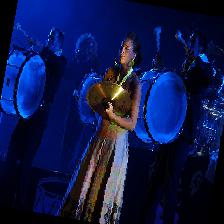}\vspace{.01cm} & jellyfish & $\phi_8$ \\ \hline
IMG\_C4 & \vspace{.01cm} \includegraphics[width=0.2\columnwidth,height=0.2\columnwidth,valign=c]{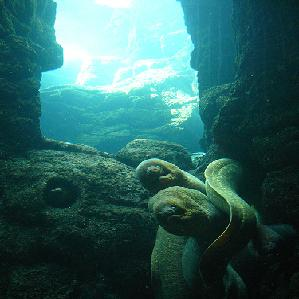}\vspace{.01cm} & \begin{tabular}[c]{@{}c@{}}sea\_snake\\ scuba\_diver\\ sea\_lion\\ coral\_reef\\ brain\_coral\end{tabular} & \vspace{.01cm} \includegraphics[width=0.2\columnwidth,height=0.2\columnwidth,valign=c]{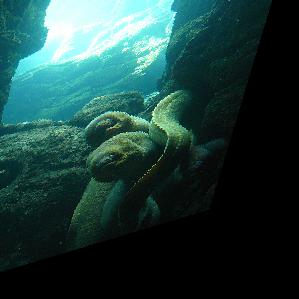}\vspace{.01cm} & wreck & $\phi_9$  \\ \hline
IMG\_C5 & \vspace{.01cm}  \includegraphics[width=0.2\columnwidth,height=0.2\columnwidth,valign=c]{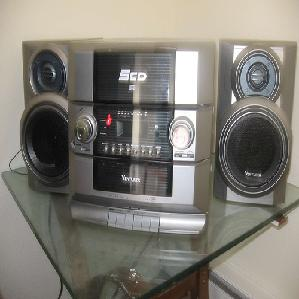}\vspace{.01cm} & \begin{tabular}[c]{@{}c@{}}cassette\_player\\ tape\_player\\ radio\\ CD\_player\\ loudspeaker\end{tabular} & \vspace{.01cm} \includegraphics[width=0.2\columnwidth,height=0.2\columnwidth,valign=c]{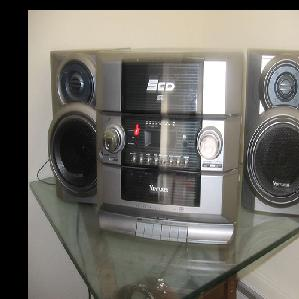}\vspace{.01cm} & Polaroid\_camera & $\phi_{11}$  \\ \hline
IMG\_C6 & \vspace{.01cm}  \includegraphics[width=0.2\columnwidth,height=0.2\columnwidth,valign=c]{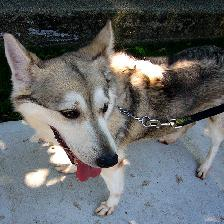}\vspace{.01cm} & \begin{tabular}[c]{@{}c@{}}Eskimo\_dog\\ Siberian\_husky\\ malamute\\ Norwegian\_elkhoun\\ Pembroke\end{tabular} & \vspace{.01cm} \includegraphics[width=0.2\columnwidth,height=0.2\columnwidth,valign=c]{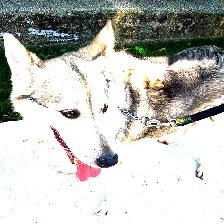}\vspace{.01cm} & Cardigan & $\phi_5$ \\ \hline
API\_C1 & \vspace{.01cm}  \includegraphics[width=0.2\columnwidth,height=0.2\columnwidth,valign=c]{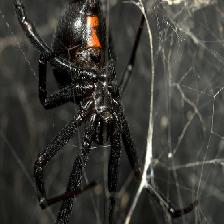}\vspace{.01cm} & \begin{tabular}[c]{@{}c@{}}spider\\ arachnid\\ invertebrate\\ tangle\_web\_spider\\ arthropod\end{tabular} & \vspace{.01cm} \includegraphics[width=0.2\columnwidth,height=0.2\columnwidth,valign=c]{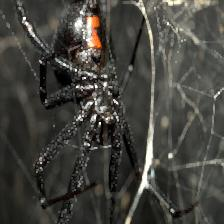}\vspace{.01cm} & water & $\phi_{3}$ \\ \hline
API\_C2 & \vspace{.01cm}  \includegraphics[width=0.2\columnwidth,height=0.2\columnwidth,valign=c]{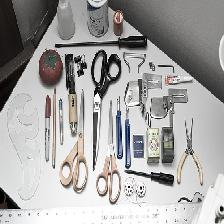}\vspace{.01cm} & \begin{tabular}[c]{@{}c@{}}scissors\\ equipment\\ tool\\ steel\\ work\end{tabular} & \vspace{.01cm} \includegraphics[width=0.2\columnwidth,height=0.2\columnwidth,valign=c]{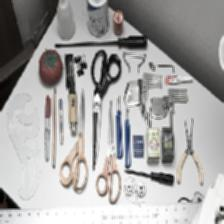}\vspace{.01cm} & business & $\phi_{1}$ \\ \hline
API\_C3 & \vspace{.01cm}  \includegraphics[width=0.2\columnwidth,height=0.2\columnwidth,valign=c]{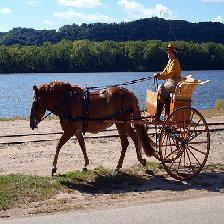}\vspace{.01cm} & \begin{tabular}[c]{@{}c@{}}carthorse\\ odd-toed\_ungulate\\ mammal\\ animal\\ buggy\end{tabular} & \vspace{.01cm} \includegraphics[width=0.2\columnwidth,height=0.2\columnwidth,valign=c]{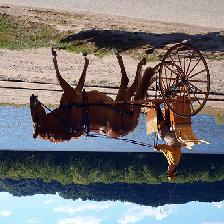}\vspace{.01cm} & elk & $\phi_{12}$ \\ \hline
API\_C4 & \vspace{.01cm}  \includegraphics[width=0.2\columnwidth,height=0.2\columnwidth,valign=c]{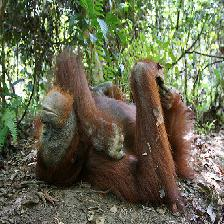}\vspace{.01cm} & \begin{tabular}[c]{@{}c@{}}tree\\ outdoor\\ animal\\ mammal\\ ape\end{tabular} & \vspace{.01cm} \includegraphics[width=0.2\columnwidth,height=0.2\columnwidth,valign=c]{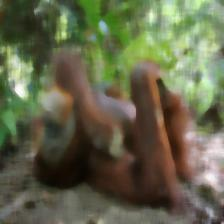}\vspace{.01cm} & fungus & $\phi_2$ \\ \hline
API\_C5 &  \includegraphics[width=0.2\columnwidth,height=0.2\columnwidth,valign=c]{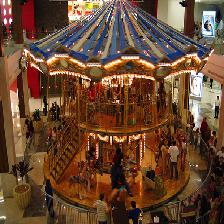}\vspace{.05cm} & \begin{tabular}[c]{@{}c@{}}Belt\\ Carousel\\ Indoors\\ Lobby\\ Reception\end{tabular} & \includegraphics[width=0.2\columnwidth,height=0.2\columnwidth,valign=c]{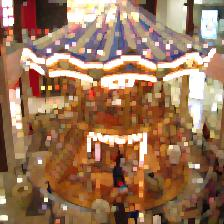}\vspace{.05cm} & architecture & $\phi_4$ \\
\end{tabular}
\end{table*}

\end{appendix}
